# Supplementary material for: The BitTorrent Anonymity Marketplace
Source: arXiv:1108.2718 source file (2011-08-12)
Supplement: Supplementary file 1 [file impl_details_appendix.tex]

For the interested reader, we provide some additional details about our
BitTorrent Marketplace Implementation.

\paragraph{DHT Messages.} The DHT responds to the following four client messages:
\begin{enumerate}
\item \textbf{Torrent List} - The DHT transmits the complete list of torrents currently
advertised in the Marketplace.
\item \textbf{Peers List} - The DHT transmits a random subset of nodes actively
participating in a specific torrent.
\item \textbf{Active} - The DHT records that the client is active in a given torrent. This
is used for the first time a node joins the torrent, and also as a heartbeat message.
Nodes are removed periodically.
\item \textbf{Drop Torrent} - The DHT removes the client from the list of nodes
participating in the torrent.
\end{enumerate}   

These functions could obviously be carried out by a slightly modified Tracker. However,
given the nature of the Anonymity Marketplace, a DHT might be the more appropriate 
vehicle for managing this information. Centralized trackers are more prone to hostile 
legal action and the like. On the other hand, while DHTs are more robust to failures,
and more resistant to legal pressures, they have non-trivial security and performance.

\paragraph{Initial Peer Connections.} When a node first connects to a peer, they
exchange a \texttt{Handshake} message for \textit{each} torrent they are
trading. If the two nodes only overlap on one torrent, and they both have active sets
of size $k$, they will initially form $2k-1$ connections. However, after an initial
exchange of metadata, connections they do not have in common are dropped.

\paragraph{Determining Peer Composition.} When adding peers to the neighborhood, a node
must decide which torrent from its active set it wishes to draw them from. Our algorithm is to
draw nodes from a torrent proportional to the value of that torrent. When the node first joins
the Marketplace, all torrents values are zero, so every torrent contributes an equal number of
peers.

\paragraph{Updating the Active Set.} At a specified interval, the node drops its least valuable torrent
for a more valuable one if one exists. Significantly, a node's native interest can drop out of the active set. 
This is important because it means that an observer cannot be absolutely certain that a node's current active set contains its native 
interest. To facilitate finding better torrents and cycling the native interest back into activity, when updating the
active set, the node can choose to occasionally chose a random torrent to cycle into activity. This is
analogous to an optimistic unchoke. In value terms, it can be seen as an investment. Even if the node
detects no significant activity in the selected torrent, \textit{its} activity in the torrent may increase
its value and draw other nodes into participation. Incidentally, this behavior is sometimes
seen in real-world stock markets and is called a \textit{self-fulfilling prophecy}.
